# Supplementary material for: OccInpFlow: Occlusion-Inpainting Optical Flow Estimation by Unsupervised Learning
Source: arXiv:2006.16637 source file (2020-06-30)

# Feature Extractor

$$I_1^i \quad H \times W \times 2$$

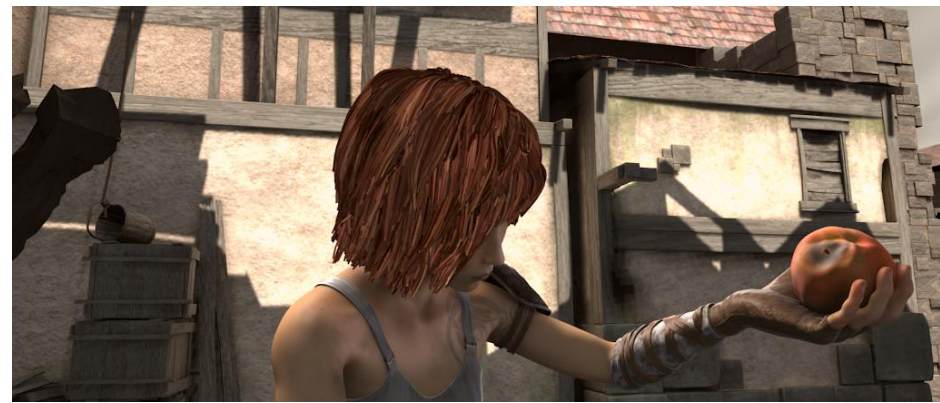

$$M_f^i \quad H \times W \times 1$$

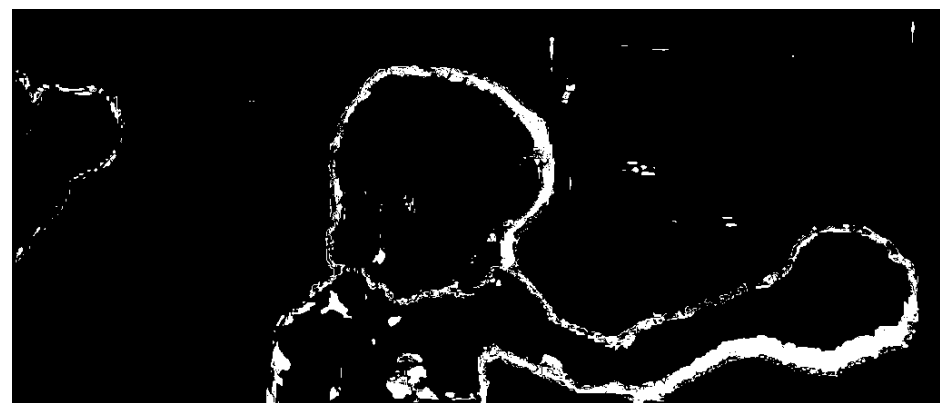

$$\hat{F}_1^i \quad H \times W \times 32$$

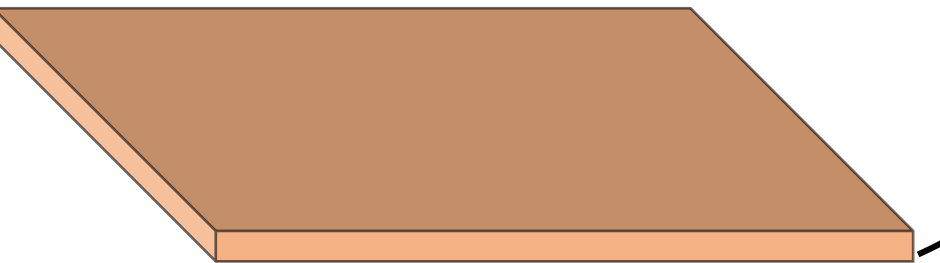

$$A_f^i \quad H \times W \times 2$$

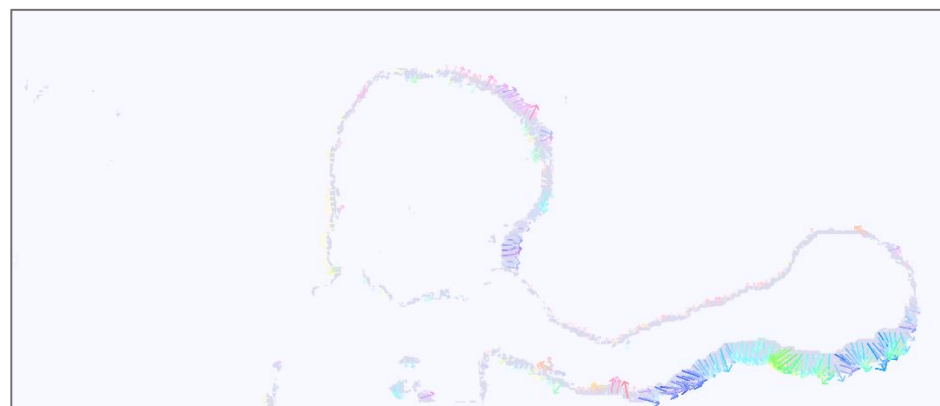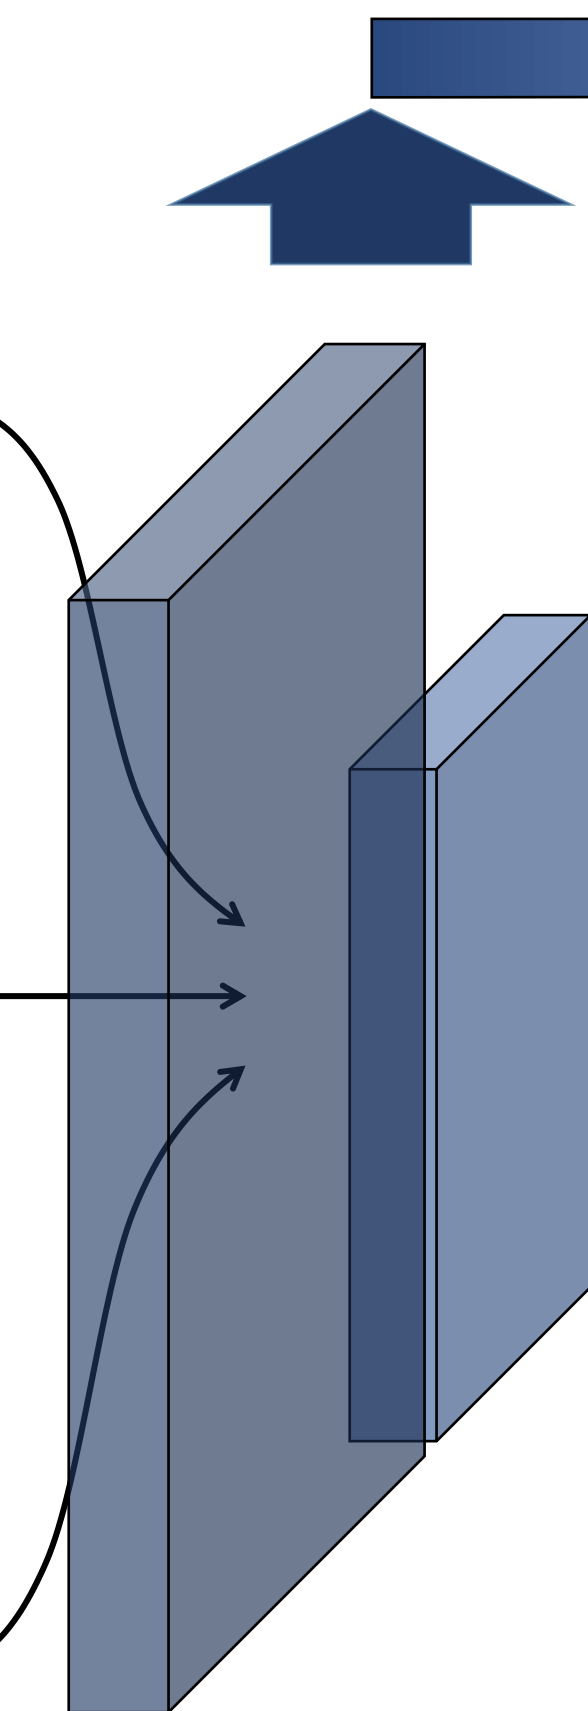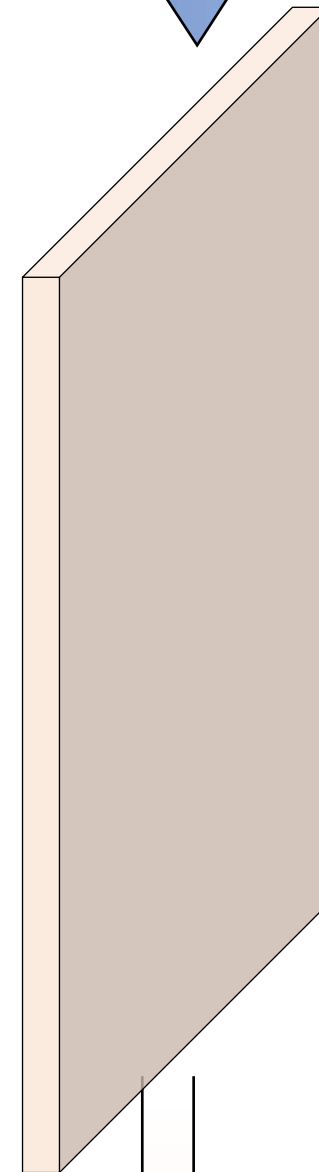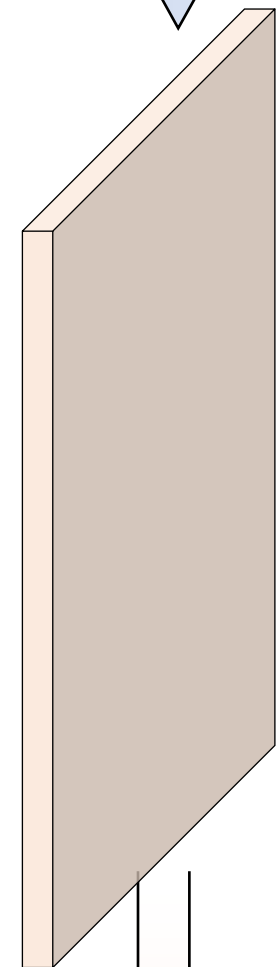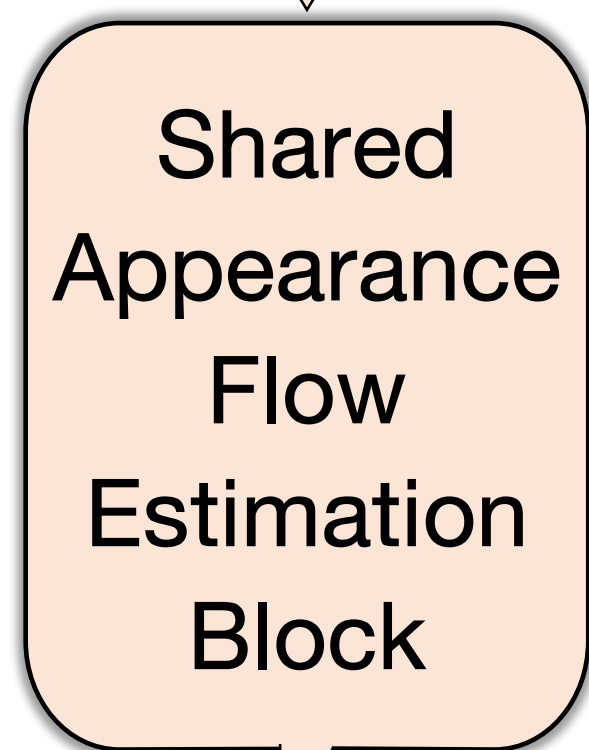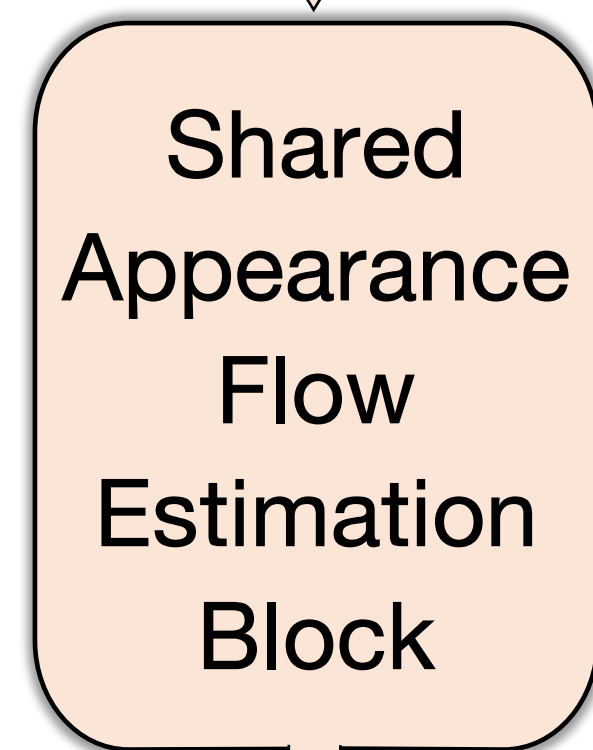

$init = 0$

# Feature Extractor

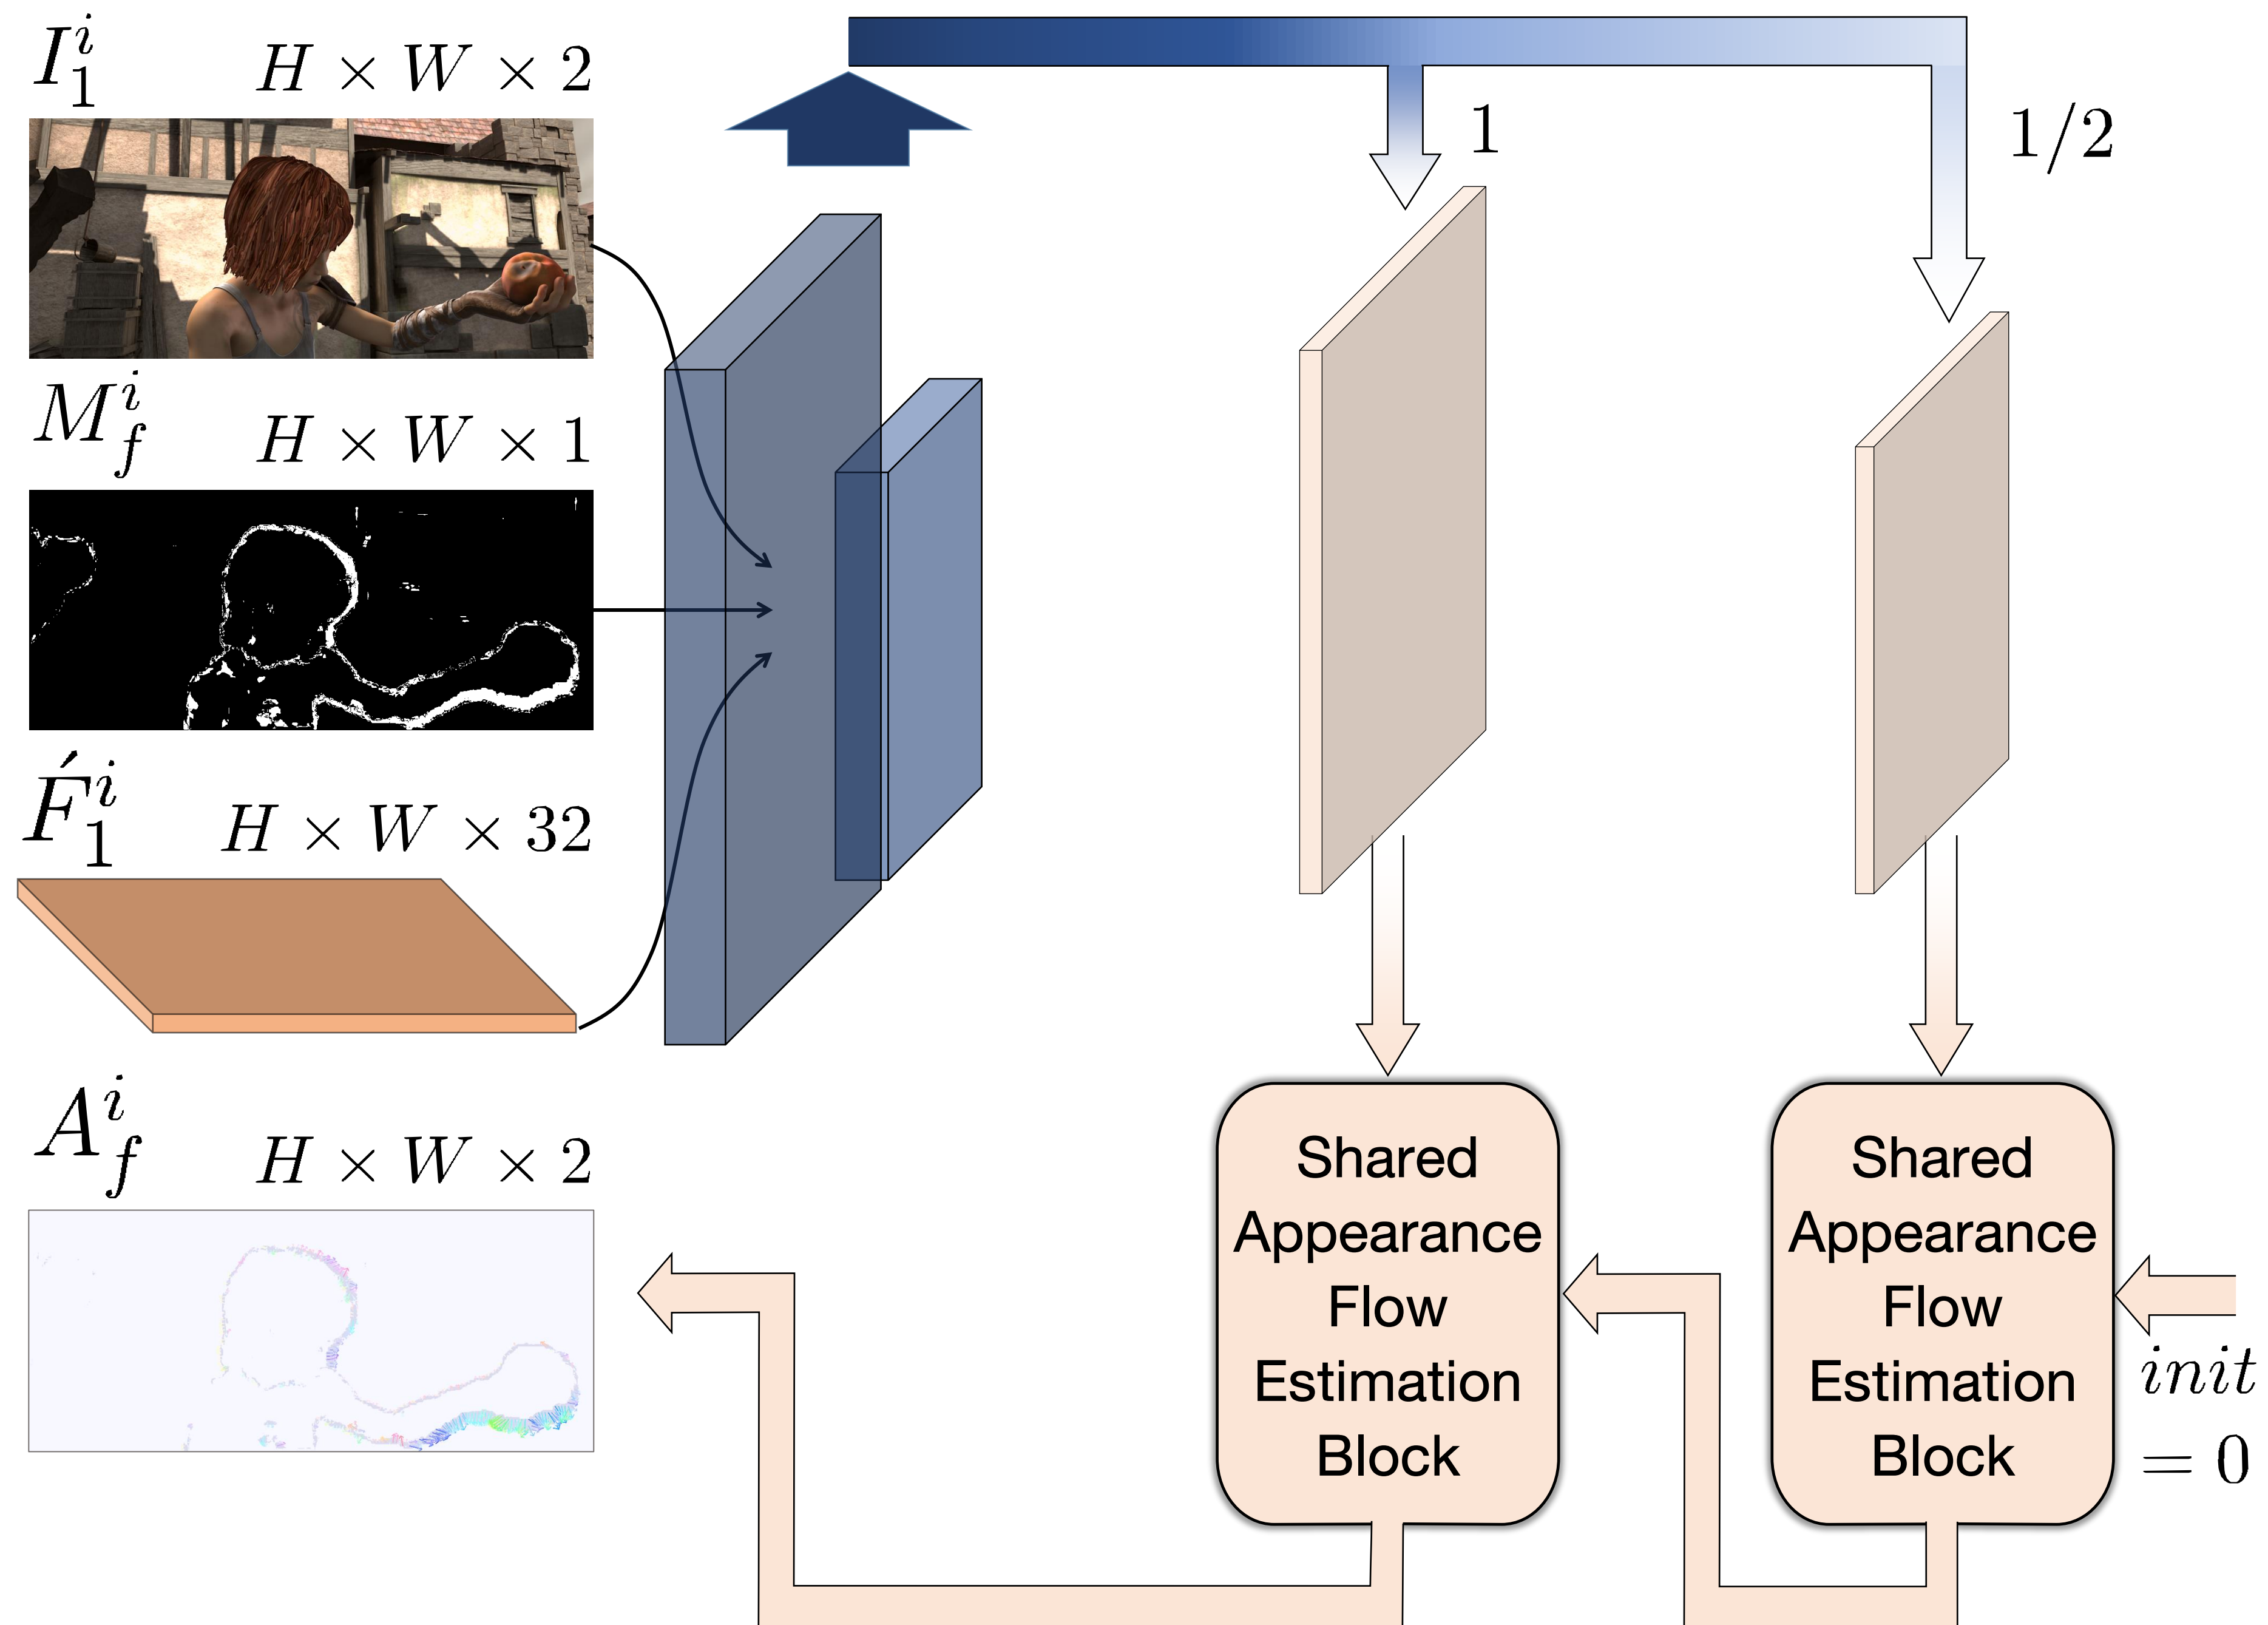

Supplement: Supplementary file 1 [file AppFlowNet_Lite.pdf]
